# Supplementary material for: An Efficient Closed-Form Method for Optimal Hybrid Force-Velocity Control
Source: arXiv:2011.04872 source file (2021-03-24)
Supplement: Supplementary file 1 [file APPENDIX.tex]

% !TEX root = ../ICRA2019Hybrid.tex

\section*{APPENDIX}

Appendixes should appear before the acknowledgment.
